# Supplementary material for: Fractal forcing of turbulence by settling particles
Source: arXiv:2610.26050 source file (2026-10-19)
Supplement: Supplementary file 1 [file appendix.tex]

\setcounter{table}{0}
\makeatletter 
\renewcommand{\thetable}{A\@arabic\c@table}
\makeatother

\setcounter{figure}{0}
\makeatletter 
\renewcommand{\thefigure}{A\@arabic\c@figure}
\makeatother

\setcounter{equation}{0}
\makeatletter 
\renewcommand{\theequation}{A\@arabic\c@equation}
\makeatother

%%%%%%%%%%%%%%%%%%%%%%%%%%%%%%%%%%%%%%%%%%%%%%%%%%%%%%%%%%%%%%%%%%%%


\begin{appen}
\vspace{-8pt}
\section{Lower volume fractions}\label{app:phi1}
\begin{figure*}[ht!]
  \centering
  \begin{subcaptiongroup}
    \begin{overpic}[width=\linewidth]{Figures/panel3_02.pdf}
      \subcaptionlistentry{}
      \label{fig:ekx-phi1}
      \put(07,63){\captiontext*{}}

      \subcaptionlistentry{}
      \label{fig:voropdfall}
      \put(50,63){\captiontext*{}}

      \subcaptionlistentry{}
      \label{fig:cfor10phi1}
      \put(07,31)  {\captiontext*{}}

      \subcaptionlistentry{}
      \label{fig:cfor100phi1}
      \put(50,31){\captiontext*{}}
    \end{overpic}
  \end{subcaptiongroup}
  \captionsetup{subrefformat=parens}
  \caption{Results for $\phi=0.01$:
  \subref{fig:ekx-phi1}~Vertical ($E_\ver$, {\protect\mycontline}) and horizontal ($E_\rad$,{\protect\mydottedline}) energy spectra in $\krad$. \subref{fig:voropdfall}~Distribution of Voronoi volumes, with the $\phi=0.10$ distributions shown in semitransparency for comparison. In the inset, we report the Voronoi cluster distribution for both $\phi=0.01, 0.10$ cases based on the alternative cluster definition discussed in \S\ref{app:phi1}.  \subref{fig:cfor10phi1}-\subref{fig:cfor100phi1}~$\mathcal{P}_\ver(\krad)$ for $\rhoratio=10$ \subref{fig:cfor10phi1} and $100$ \subref{fig:cfor100phi1}.}
  \label{fig:fig1e}
\end{figure*}


To assess the effect of dilution on CIT, we here analyze two lower-volume-fraction cases ($\phi=0.01$, with $\rhoratio=10, 100$). As for the $\phi=0.10$ cases, the scale-by-scale energy spectra (\cref{fig:ekx-phi1}) shows low-wavenumber energy accumulation, hallmark of CIT. However, the Voronoi-volume distributions (\cref{fig:voropdfall}) are so close to the random reference distribution that it is not possible to identify clustered particles under the standard definition of \cite{monchaux-bourgoin-ea2010}. Nevertheless, even in uniformly random distributions, local density variations are known to generate large-scale fluctuations in gravity-forced flows \citep{hinch1988,tandurella-rosti-ea2026}.  To capture these active variations is sufficient to use a broader cluster definition: a simple option is to classify a particle as clustered if its Voronoi volume $V_v$ is less than the mean Voronoi volume $\Vdp/\phi = V_D/\ndp$. 
Applying the same clustering procedure described in the main text, we can identify clusters even at $\phi=0.01$; their volume distributions (inset of \cref{fig:voropdfall}) remain self-similar and steeper than $V_\cluster^{-2}$. The spectral cluster decomposition (\cref{eq:clusterdecomp}, \cref{fig:cfor10phi1,fig:cfor100phi1}) shows a distinct low-wavenumber peak that matches the large-scale kinetic energy increase seen in \cref{fig:ekx-phi1}. Notably, clustered particles remain solely responsible for the large-scale forcing, but the underlying hierarchical structure is fundamentally altered: unlike the $\phi=0.10$ cases, the large-scale energy injection is no longer dominated by the primary $C_1$, but instead emerges as a collective sum of contributions from multiple smaller clusters. 
This analysis shows that in dilute conditions cluster-induced fluctuations remain present, despite not showing a developed self-similar regime seen at higher $\phi$. Extension to larger domains will be needed to better understand the large-scale power injection.

\end{appen}
